# Supplementary material for: Semantic Topic Analysis of Traffic Camera Images
Source: arXiv:1809.10707 source file (2018-09-27)
Supplement: Supplementary file 1 [file appendix.tex]

\begin{figure}[htb]
\centering
\includegraphics[width=\linewidth]{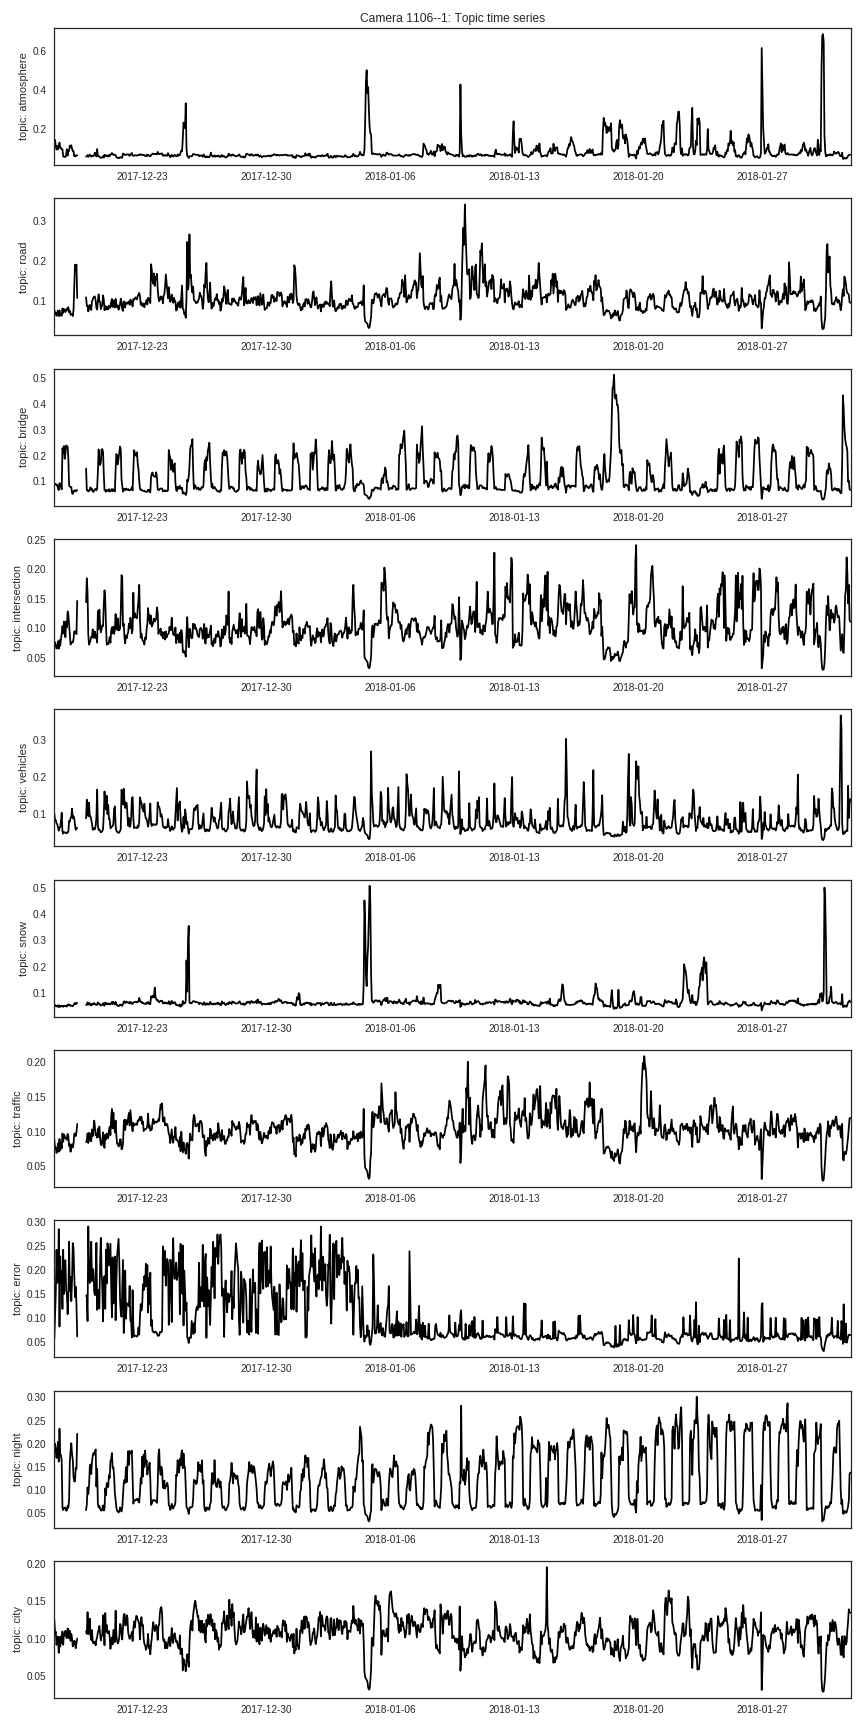}
\caption{Camera 1106--1}
\label{fig:ts_1106}
\end{figure}
\begin{figure}[htb]
    \centering
\includegraphics[width=\linewidth]{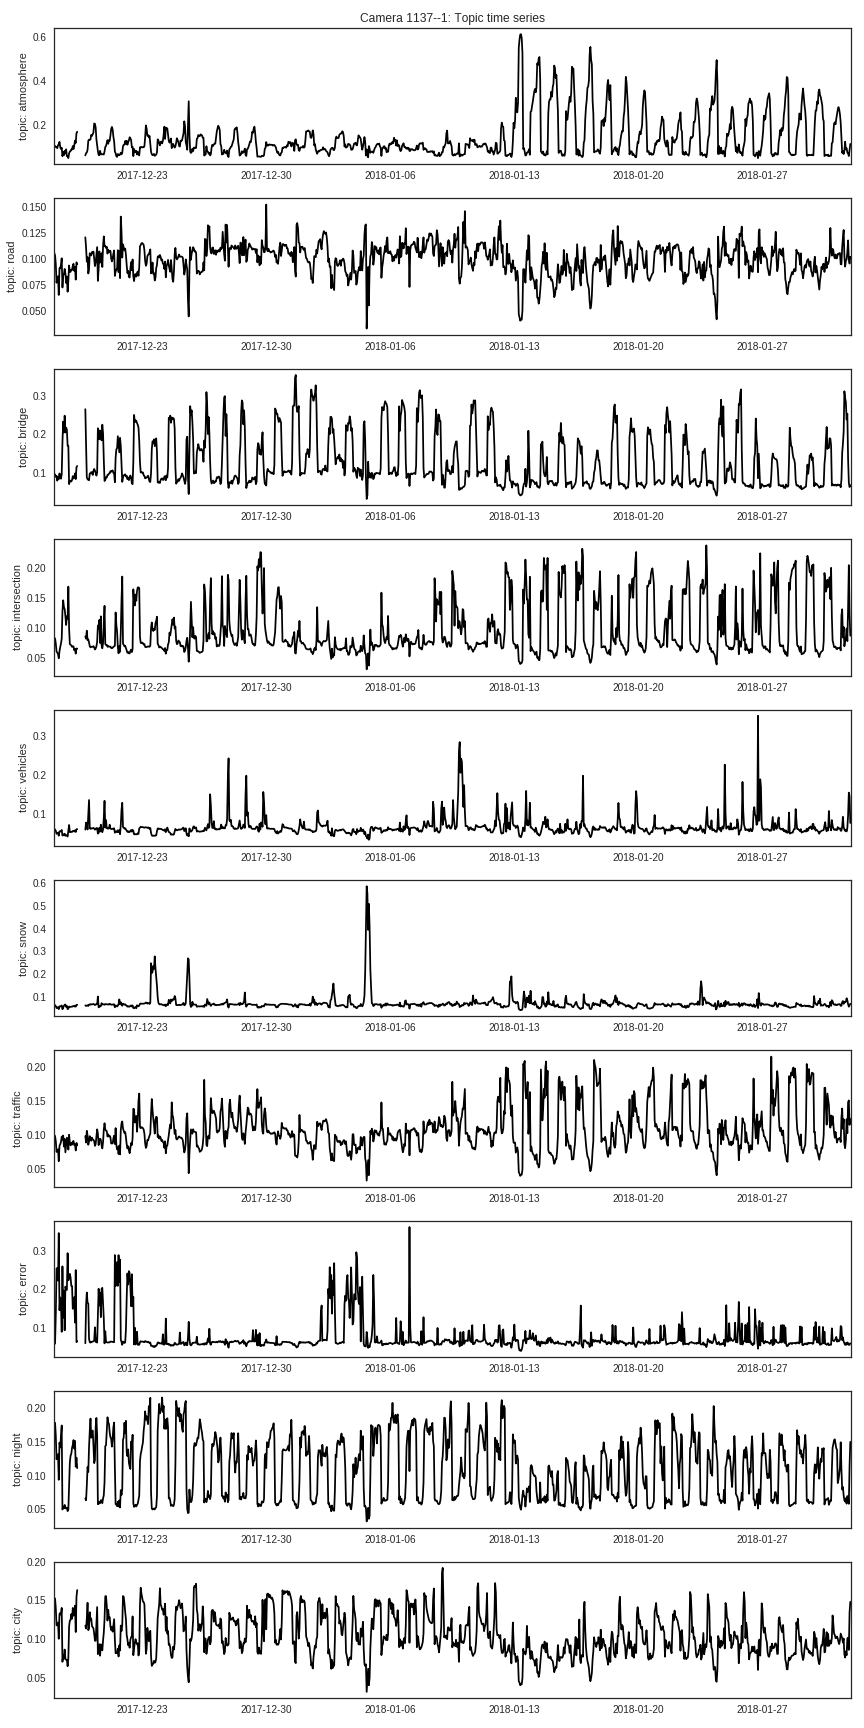}
\caption{Camera 1137--1}
\label{fig:ts_1137}
\end{figure}
\begin{figure}[htb]
    \centering
\includegraphics[width=\linewidth]{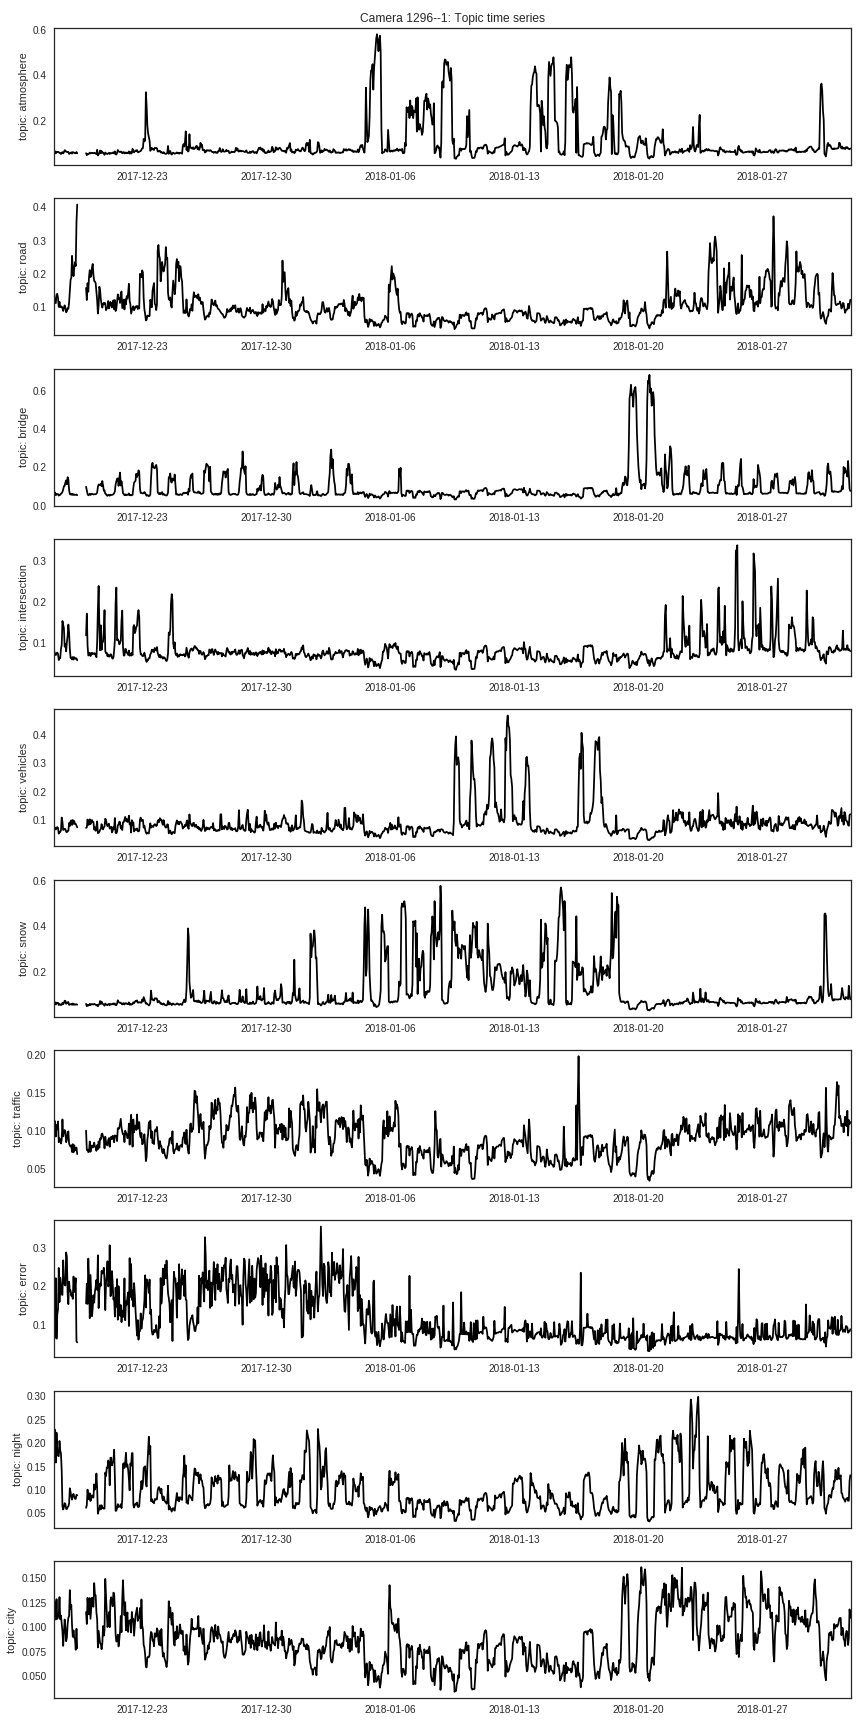}
\caption{Camera 1296--1}
\label{fig:ts_1296}
\end{figure}
\begin{figure}[htb]
    \centering
\includegraphics[width=\linewidth]{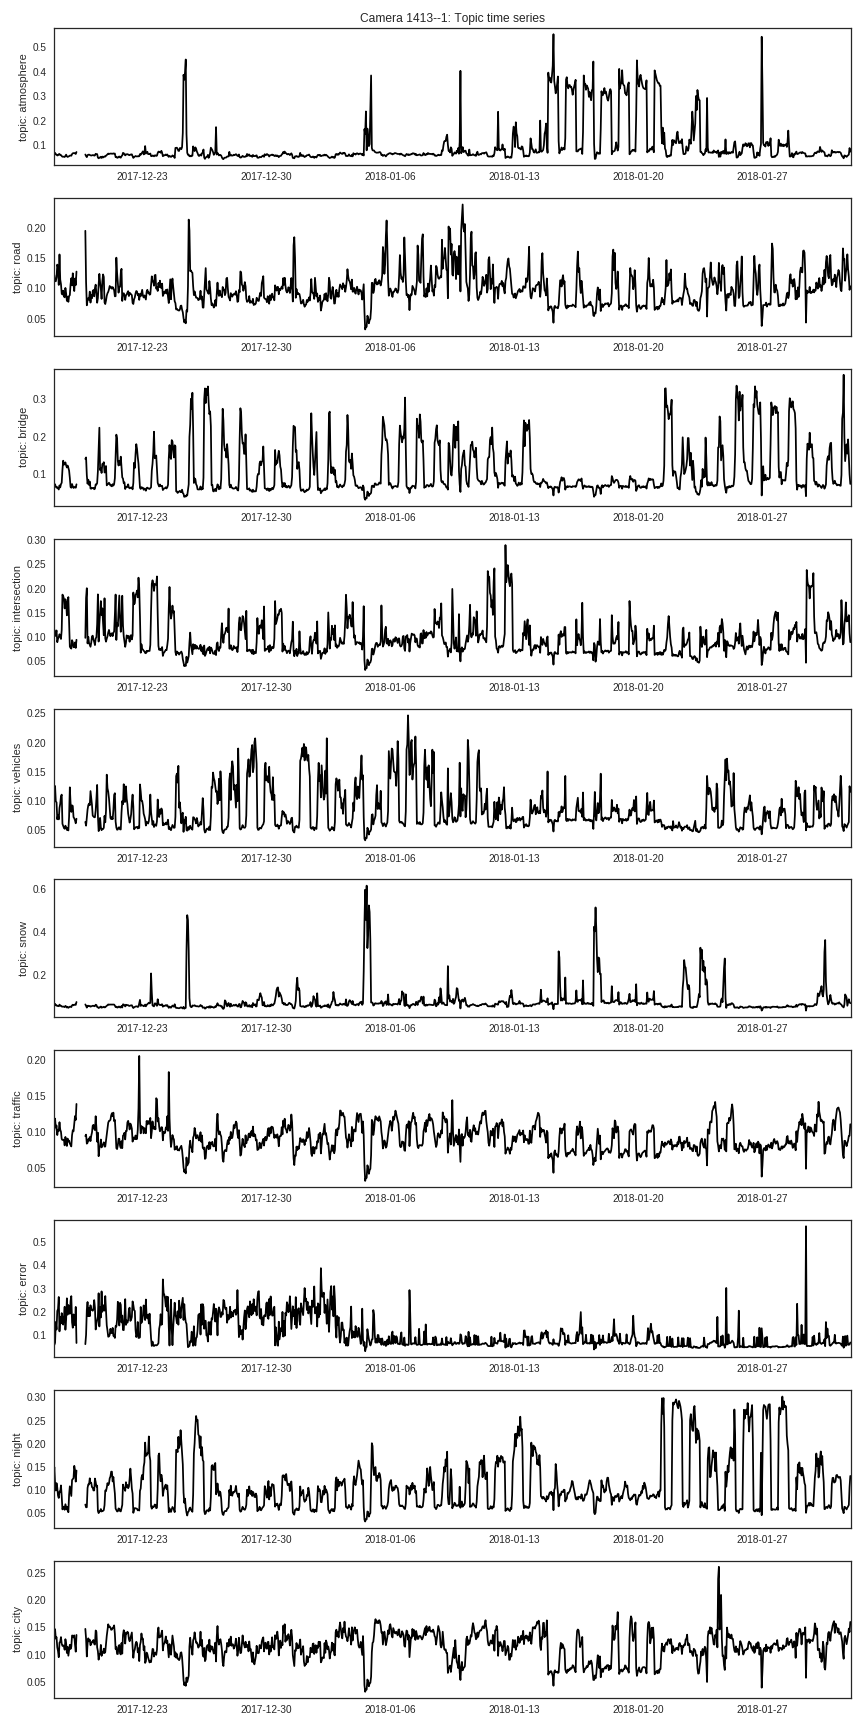}
\caption{Camera 1413--1}
    \label{fig:ts_1413}
\end{figure}
\begin{figure}[htb]
    \centering
    \includegraphics[width=\linewidth]{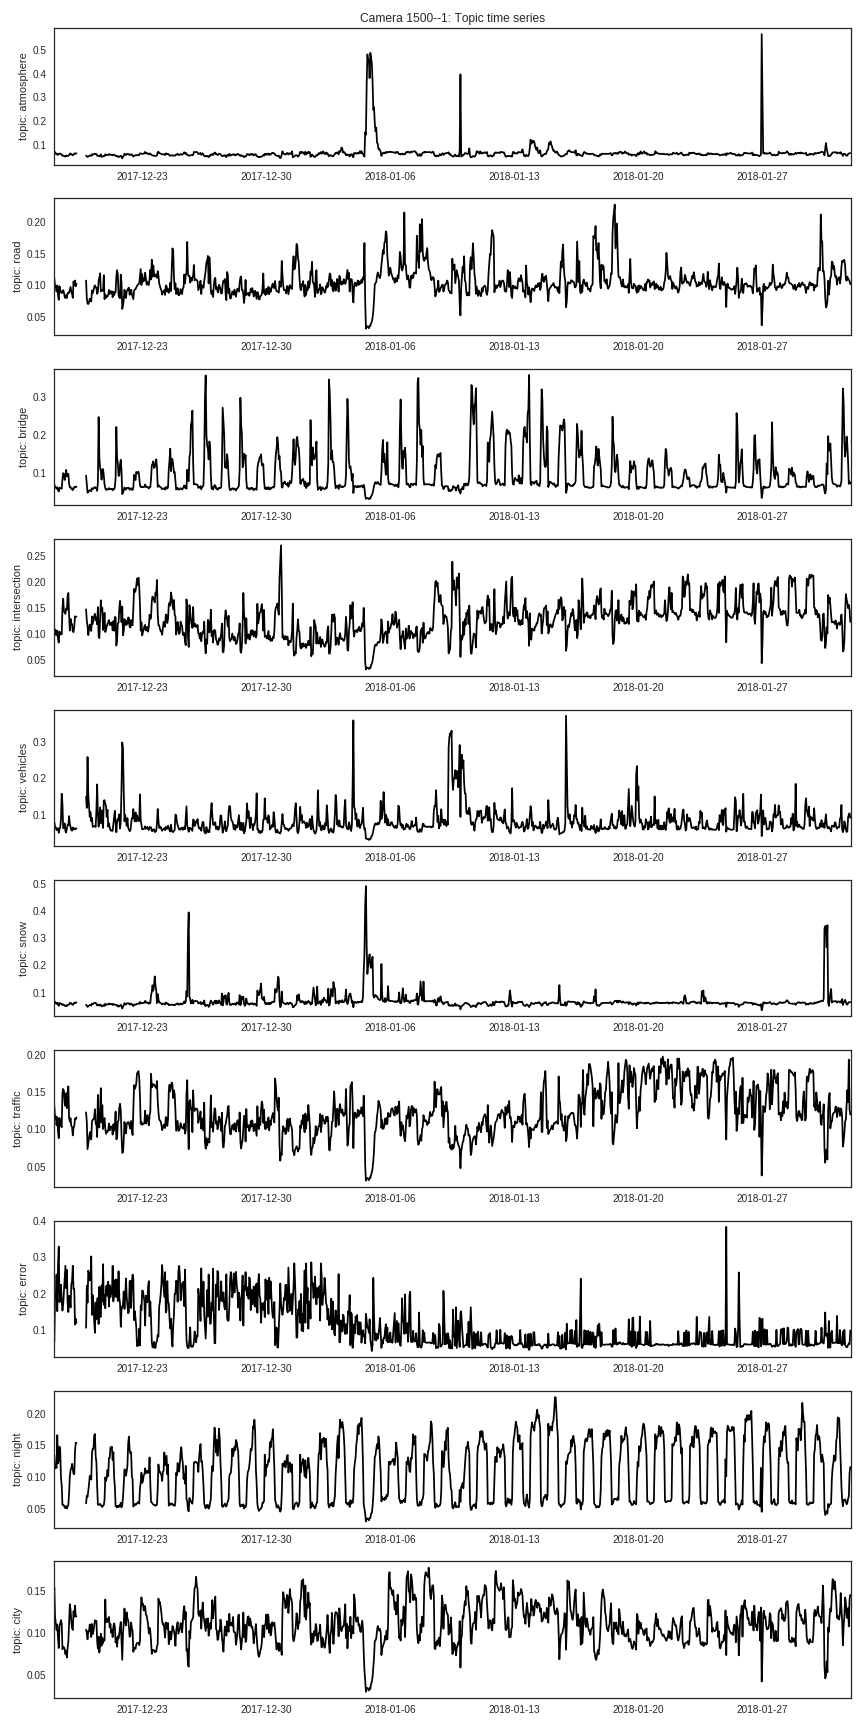}
    \caption{Camera 1500--1}
    \label{fig:ts_1500}
\end{figure}
\begin{figure}[htb]
    \centering
    \includegraphics[width=\linewidth]{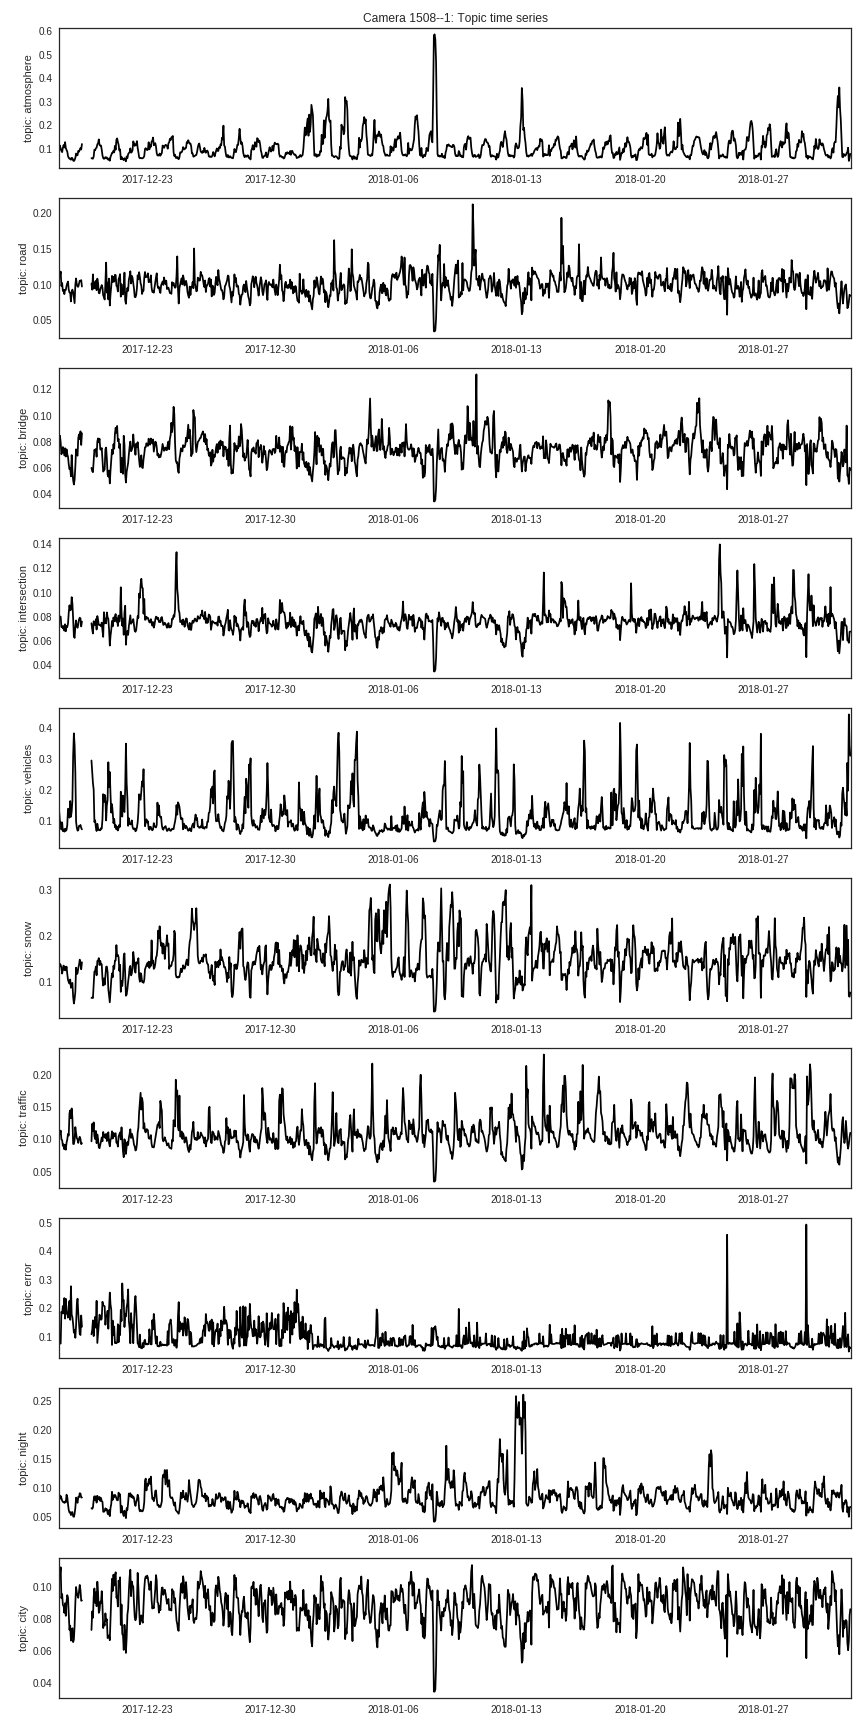}
    \caption{Camera 1508--1}
    \label{fig:ts_1508}
\end{figure}
\begin{figure}[htb]
    \centering
    \includegraphics[width=\linewidth]{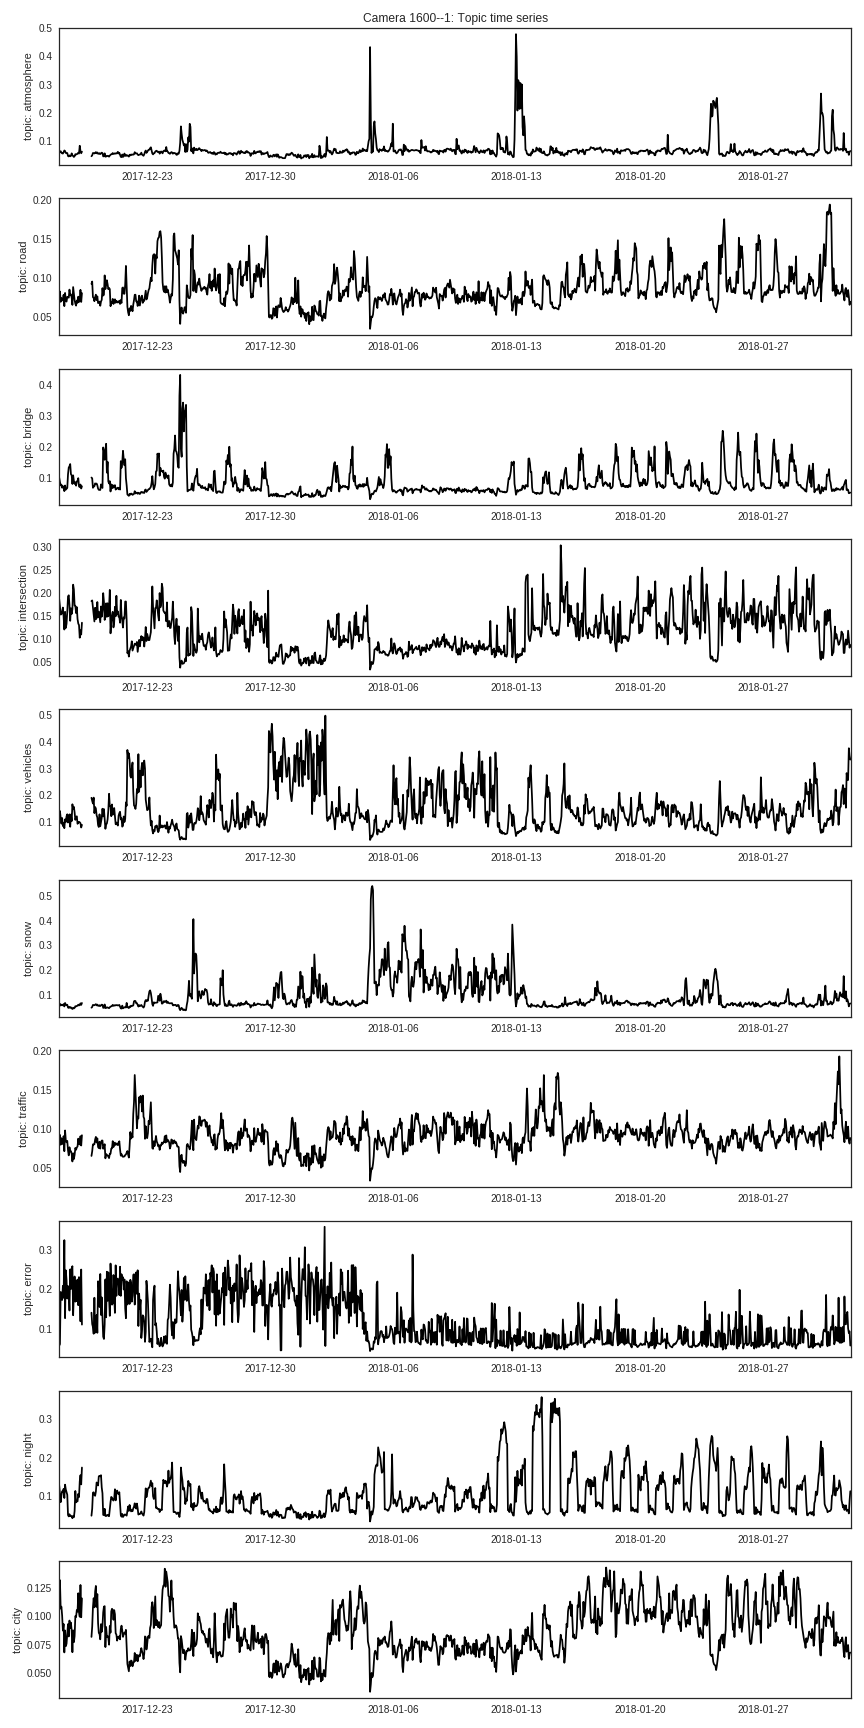}
    \caption{Camera 1600--1}
    \label{fig:ts_1600}
\end{figure}
